# Supplementary material for: Closed form Eigenvalues of Randomly Segmented Tridiagonal quasi-Toeplitz Matrices: Random Rouse block copolymer
Source: arXiv:2202.10249 source file (2023-05-26)
Supplement: Supplementary file 1 [file supplement.pdf]

# Closed form Eigenvalues of Randomly Segmented Tridiagonal quasi-Toeplitz Matrices: Random Rouse block copolymer

S.S. Ashwin[1, 2, *]

[1] *Theoretical Biophysics Lab, Department of Applied Physics, Nagoya University, Nagoya, Japan*
[2] *Center for Computational Natural Sciences and Bioinformatics IIIT Hyderabad, Gachibowli, Hyderabad*

(Dated: May 5, 2023)

## CALCULATION $g(\tan(\tilde{\phi}_m))$ :

We will demonstrate how to calculate $g(\tan(\tilde{\phi}_m))$ which will account for $\mathcal{O}(N_m^{-1})$ corrections to $P(\lambda)$. For notational convenience, we will use $r = \tan(\tilde{\phi}_m)$. A natural choice for the distribution $P_\xi(\xi)$ is the $\chi^2(d)$ distribution, which allows for parametric tuning of the degree of freedom $d$ to a variety of distributions. If $P_\xi(\xi)$ is a $\chi^2(d)$ distribution, then $P_w(w)$ can be derived using a Melins transform [1]. While the expression for $P_w(w)$ is exact for the $\chi^2(d)$ distribution, it is very inconvenient to calculate as it involves sums of generalized hypergeometric functions. Instead, we use Fisher-Snedecor's $F$-distribution [3], which has a simpler form and is a good approximation [4].

We choose the probability distribution of sizes to be normal, $P_n(n) = \sqrt{\pi/\alpha_o} e^{-\alpha(n-n_o)^2}$, with a large $\alpha$. Using this, a simple iteration over (1) quickly converges to a solution of $g(r)$.

$$g(r) = \int_{-\infty}^{\infty} g(r') \left\langle \frac{P_w\left(w^*\right)}{\gamma'(r', w^*, n)} \right\rangle_n dr' \tag{1}$$

$$w* = \frac{r\mathcal{U}_n + rr'\mathcal{T}_{n+1}}{(\sin(k) + r\cos(k))(\mathcal{U}_{n-1} + r'\mathcal{T}_n)}$$

Shown in Fig(1) is the converged solution $g(r)$ with different $n$ and $k$ for $\chi^2(2)$. Note, the $g(r)$ is thinly distributed for small $k$ while it becomes larger at larger $k$.

* ss.ashwin@gmail.com

[1] Melvin Dale, "The Algebra of Random variables", Wiley, New York, (1979).

[2] S.B. Provost, E. M. Rudiuck, Ann. Inst. Statist. Math, **46**;3, 557-571, (1993).

[3] C. Walck, "Handbook on statistical distributions for experimentalists," Particle Phys. Group, Fysikum, Univ. Stockholm, Sweden, (2007).

[4] B. Epstien, Ann. Math. Statist. **19(3)**, 370-379 (1948).

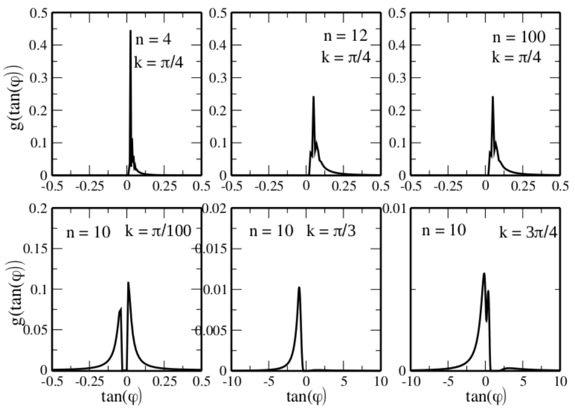


Figure 1. Distributution of $g(\tan(\tilde{\phi}))$ *vs* $\tilde{\phi}$ for $n$ and $k$ indicated. With distribution $P_\xi(\xi) = \chi^2(2)$.
